# Supplementary material for: Coexistence of ferromagnetism and superconductivity in iron based pnictides: a time resolved magnetooptical study
Source: arXiv:1410.4651 source file (2014-10-17)
Supplement: Supplementary file 1 [file TR-Eu-122-sr-supplemental.pdf]

# Coexistence of ferromagnetism and superconductivity in iron based pnictides: a time resolved magnetooptical study (supplemental information)

A. Pogrebna,[1,2] T. Mertelj,[1] N.Vujičić,[1,3] G. Cao,[4] Z. A. Xu,[4] and D. Mihailovic[1,5]

[1] *Complex Matter Dept., Jozef Stefan Institute, Jamova 39, SI-1000 Ljubljana, Slovenia*

[2] *Jožef Stefan International Postgraduate School, Jamova 39, SI-1000 Ljubljana, Slovenia*

[3] *Institute of Physics, Bijenička 46, HR-10000 Zagreb, Croatia*

[4] *Department of Physics, Zhejiang University, Hangzhou 310027, People's Republic of China*

[5] *CENN Nanocenter, Jamova 39, SI-1000 Ljubljana, Slovenia*

(Dated: October 2, 2014)

**Contents**

**Optical response in the conical helimagnetic state** 1

**Optical response in the canted antiferromagnetic state** 2

**References** 2

## Optical response in the conical helimagnetic state

Assuming that within a single plane $Eu^{2+}$ spins are ordered ferromagnetically Eq. (1) can be applied to each plane separately. Neglecting for simplicity the crystallographic details and assuming a conical helimagnetic phase with $\mathbf{M} = M_0[\cos(q_0 z)\sin(\theta), \sin(q_0 z)\sin(\theta), \cos(\theta)]$, where $q_0$ represents the helix propagation wavevector and $\theta$ the local magnetization angle relative to the $c$-axis, we introduce following Ref. [1] a local coordinate system,

$$\begin{aligned}\hat{x}' &= [\hat{x}\cos(q_0 z) + \hat{y}\sin(q_0 z)]\cos(\theta) - \hat{z}\sin(\theta),\\ \hat{y}' &= -\hat{x}\sin(q_0 z) + \hat{y}\cos(q_0 z),\\ \hat{z}' &= [\hat{x}\cos(q_0 z) + \hat{y}\sin(q_0 z)]\sin(\theta) + \hat{z}\cos(\theta).\end{aligned} \tag{S1}$$

Here ˆ represents the Cartesian unit vectors. The modes of a spin-operators linearized Hamiltonian are then represented by,[2]

$$\begin{aligned}\delta M_{x'}(z) &\propto \sum_m s_{x'}(\mathbf{q} + m q_0 \hat{z}) e^{i[(\mathbf{q}+m q_0 \hat{z})\cdot\mathbf{r} - \omega(\mathbf{q})t]},\\ \delta M_{y'}(z) &\propto \sum_m s_{y'}(\mathbf{q} + m q_0 \hat{z}) e^{i[(\mathbf{q}+m q_0 \hat{z})\cdot\mathbf{r} - \omega(\mathbf{q})t]},\end{aligned} \tag{S2}$$

where $m$ are integers and $s_{i'}(\mathbf{q})$ and $\omega(\mathbf{q})$ depend on the particular choice of Hamiltonian.[1, 2] Here nonzero $m$ terms need to be introduced because in the presence of an in-plane external magnetic field higher harmonics appear in the modulation.[2] An in-plane anisotropy also introduces higher harmonic terms. Transforming back to the crystal coordinate system and taking into account only the oscillating part by omiting the terms containing $\delta M_{z'}$ we obtain:

$$\begin{aligned}\delta M_x(z) &\propto e^{-i\omega(\mathbf{q})t}\cos(\theta)[\cos(q_0\hat{z})\sum_m s_{x'}(\mathbf{q}+mq_0\hat{z})e^{i(\mathbf{q}+mq_0\hat{z})\cdot\mathbf{r}} - \sin(q_0\hat{z})\sum_m s_{y'}(\mathbf{q}+mq_0\hat{z})e^{i(\mathbf{q}+mq_0\hat{z})\cdot\mathbf{r}}],\\ \delta M_y(z) &\propto e^{-i\omega(\mathbf{q})t}\cos(\theta)[\sin(q_0\hat{z})\sum_m s_{x'}(\mathbf{q}+mq_0\hat{z})e^{i(\mathbf{q}+mq_0\hat{z})\cdot\mathbf{r}} + \cos(q_0\hat{z})\sum_m s_{y'}(\mathbf{q}+mq_0\hat{z})e^{i(\mathbf{q}+mq_0\hat{z})\cdot\mathbf{r}}],\\ \delta M_z(z) &\propto e^{-i\omega(\mathbf{q})t}\sin(\theta)\sum_m s_{x'}(\mathbf{q}+mq_0\hat{z})e^{i(\mathbf{q}+mq_0\hat{z})\cdot\mathbf{r}}.\end{aligned} \tag{S3}$$

$\langle M_i \delta M_i \rangle$ therefore contains terms:

$$\langle M_x\delta M_x\rangle \propto \cos^2(\theta)\sum_m s_{x'}(q_z\hat{z}+mq_0\hat{z})\langle\cos^2(q_0z)e^{i(q_z+mq_0)z}\rangle,$$
$$\langle M_y\delta M_y\rangle \propto \cos^2(\theta)\sum_m s_{x'}(q_z\hat{z}+mq_0\hat{z})\langle\sin^2(q_0z)e^{i(q_z+mq_0)z}\rangle,$$
$$\langle M_z\delta M_z\rangle \propto \cos(\theta)\sin(\theta)\sum_m s_{x'}(q_z\hat{z}+mq_0\hat{z})\langle e^{i(q_z+mq_0)z}\rangle. \quad \text{(S4)}$$

Here $\langle\rangle$ represents the average over $Eu^{2+}$ planes. $\langle M_x\delta M_x\rangle$ and $\langle M_y\delta M_y\rangle$ are nonzero only when (i) $q_z+mq_0=\pm 2q_0$ or (ii) $q_z+mq_0=0$. In case (i) $\langle M_x\delta M_x\rangle=-\langle M_y\delta M_y\rangle$ leading to an anisotropic in-plane response while in case (ii) $\langle M_x\delta M_x\rangle=\langle M_y\delta M_y\rangle$ leading to the isotropic response. The frequencies present in the in-plane isotropic response are therefore $\omega(0+mq_0)$.

Due to terms $\langle e^{i(q_z+mq_0)z}\rangle$ the term $\langle M_z\delta M_z\rangle$ also leads to isotropic response at frequencies $\omega(0+mq_0)$.

The TR-MOKE response, on the other hand, is determined by $\delta\epsilon_{xy}\propto i\langle\delta M_z\rangle$ and contains terms $\langle e^{i(q_z+mq_0)z}\rangle$ that are nonzero for $q_z+mq_0=0$, which is identical to (ii). In a single magnetic domain sample the in-plane isotropic modes should therefore appear also in the $c$-axis TR-MOKE response.

## Optical response in the canted antiferromagnetic state

For convenience we switch to the standard definition of the order parameters in weak ferromagnets.[3] Assuming that the magnetization at $H=0$ is oriented along the $c$ axis, the total magnetization displacement, $\delta\mathbf{M}$, of the quasi-FM mode would lie on an ellipse perpendicular to $\mathbf{M}$ with the AFM vector displacements, $\delta\mathbf{L}$, linear along $\mathbf{M}$, [4] while for the quasi-AFM mode $\delta\mathbf{M}$ would be linear along $\mathbf{M}$ and $\delta\mathbf{L}$ on an ellipse lying in the $xy$-plane. Looking at the symmetric part of the dielectric tensor for the orthorhombic case following Iida *et al.*[4] and assuming $\mathbf{L}||a$ and $\mathbf{H}||b$ it follows:

$$\epsilon_{ii} = \epsilon_{0,ii} + a_{iizz}M_z^2 + a_{iiyy}M_y^2 + , \\ + b_{iixx}L_x^2 + c_{iizx}M_zL_x. \quad \text{(S5)}$$

Here the terms $c_{iizx}M_zL_x$ are due to the Dzyaloshinskii-Moriya interaction and are incompatible with our samples crystallographic structure ($Fmmm$).[5] The modulation of the dielectric tensor obtained from (S5) to the linear order in displacements is given by:

$$\delta\epsilon_{ii} = 2a_{iizz}M_z\delta M_z + 2a_{iiyy}M_y\delta M_y + \\ + 2b_{iixx}L_x\delta L_x + c_{iizx}(L_x\delta M_z + M_z\delta L_x). \quad \text{(S6)}$$

For both magnetic modes the nearly-isotropic response can come from the term $2a_{iizz}M_z\delta M_z$ only since $a_{xxzz}\sim a_{yyzz}$ due to the small orthorhombicity. The nearly isotropic in-plane response can therefore only be associated with $\delta M_z$. Since both modes contribute to $\delta M_z$ at a finite in-plane magnetic field, when $\mathbf{M}$ is tilted away from the $c$-axis along the magnetic field, both should occur concurrently in the transient reflectivity response.


[1] Cooper, B. R., Elliott, R., Nettel, S., & Suhl, H. Theory of magnetic resonance in the heavy rare-earth metals. *Physical Review* **127**, 57 (1962).

[2] Cooper, B. R. & Elliott, R. J. Spin-wave theory of magnetic resonance in spiral spin structures: Effect of an applied field. *Phys. Rev.* **131**, 1043–1056 (1963).

[3] Turov, E. A., Tybulewicz, A., Chomet, S., & Technica, S. *Physical properties of magnetically ordered crystals*. Academic Press (1965).

[4] Iida, R. *et al.* Spectral dependence of photoinduced spin precession in $DyFeO_3$. *Phys. Rev. B* **84**, 064402 (2011).

[5] Nandi, S. *et al.* Coexistence of superconductivity and ferromagnetism in P-doped $EuFe_2As_2$. *Phys. Rev. B* **89**, 014512 (2014).
